# Supplementary material for: StepAudio 3 Realtime Technical Report
Source: arXiv:2609.14005 source file (2026-10-12)
Supplement: Supplementary file 1 [file appendix-audio-taxonomy.tex]

\section{Audio Understanding Taxonomy}
\label{app:audio_taxonomy}

Audio understanding spans tasks with substantially different output structures and evidence requirements. Some examples require near-verbatim linguistic recovery, while others require estimating an acoustic attribute, locating an event in time, distinguishing speakers, or integrating several weak cues into a semantic conclusion. Without an explicit organization, abundant recognition-style examples can dominate training and obscure rare but interaction-critical capabilities. We therefore organize audio-understanding supervision with a hierarchical taxonomy containing 182 fine-grained sub-capabilities.

\subsection{Capability Families}

\textbf{Lexical and linguistic content.} This family includes transcription, language and dialect recognition, code-switching, text normalization, keyword and entity recovery, and content-level question answering. Context can disambiguate acoustically similar words and preserve rare domain terms that are unlikely under a context-free language prior.

\textbf{Speaker and paralinguistic attributes.} These capabilities cover speaker count and identity relations together with speaking rate, pitch behavior, vocal effort, hesitation, laughter, breathing, sighs, and other non-verbal vocalizations. Such evidence often affects conversational intent and the appropriate response style.

\textbf{Emotion, attitude, and delivery.} Beyond coarse emotion labels, the taxonomy represents intensity, changes over time, and interactions between lexical meaning and vocal expression, including cases in which the literal transcript and the speaker's apparent attitude are not aligned.

\textbf{Acoustic events and scene context.} Environmental sounds, music, overlapping speech, channel conditions, and other non-speech events provide situational context. Tasks can require identifying an event, separating foreground from background, or explaining how an event changes the interpretation of spoken content.

\textbf{Temporal and structural analysis.} This family includes segmentation, timestamp prediction, endpoint detection, forced alignment, speaker diarization, and multi-speaker transcription. These capabilities convert an unstructured waveform into an ordered account of who produced which event and when.

\textbf{Audio-grounded integration and reasoning.} The most demanding cases combine multiple observations, for example comparing speakers, relating an acoustic event to an utterance, aggregating evidence over a long recording, rejecting an unsupported premise, or explaining a conclusion grounded only in the audio.

\subsection{Use in Data Construction and Sampling}

The taxonomy is used as an operational control surface rather than only as a descriptive label set. Multi-label assignment determines which questions can be constructed from a recording, controls sampling weights, exposes underrepresented regions, and supports capability-aware quality filtering. Coverage and rarity profiles route examples toward broad mid-training, stricter SFT selection, re-evaluation, or human refinement. The same hierarchy is used to diagnose whether improvements are concentrated in abundant recognition tasks or extend to scarce capabilities such as temporal localization, multi-speaker structure, and audio-grounded reasoning.

The capability families should not be interpreted as independent prediction heads. A single recording can simultaneously require entity recognition, emotion interpretation, speaker tracking, and temporal localization. They instead define complementary queries over a shared audio--language representation, making overlapping supervision measurable without fragmenting the deployed model into separate modules.
